# Supplementary material for: Rigid body rotation and chiral reorientation combine in filamentous E. coli swimming in low-Re flows
Source: arXiv:2508.00779 ancillary file (2026-03-09)
Supplement: Supplementary file 1 [file Bacteria_Swimming_072925_SI.pdf]

# Supporting Material for Rigid body rotation and chiral reorientation combine in elongated *E. coli* swimming in low-Re flows

Richard Z. DeCurtis, Yongtae Ahn, Jane Hill, and Sara M. Hashmi\*

## I. BACTERIA LENGTHS

Figure S1 shows a histogram of the bacteria lengths for all 254 elongated bacteria, including all wigglers and non-wigglers tracked in both the slow and fast flow rates. The lengths are normally distributed, with a few individual bacteria having  $l > 10\mu\text{m}$ . The lengths range from 2.4 to  $10.1\mu\text{m}$ , with the average length  $\langle l \rangle = 4.9 \pm 1.2\mu\text{m}$ . The error bars represent the standard deviation. Given the average radius  $r = 0.33\mu\text{m}$ , these lengths correspond to a range of aspect ratios  $e = l/2r$  between 3.6 and 15.3, with an average  $\langle e \rangle = 7.4$ .

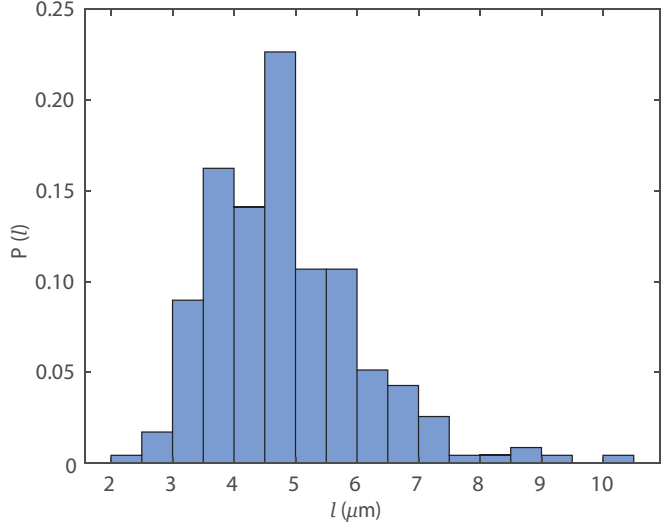

FIG. S1. Histogram  $P(l)$  for the lengths of all tracked bacteria in the microscopy videos, including both the wigglers and non-wigglers, at both flow rates.

## II. MICROSCOPY OF SWIMMING AND FLOWING BACTERIA

The SI videos are described briefly here, in the order in which they are referred to in the paper. The SI material also includes two files of raw microscopy video data, called Q=0.10-cephalexin.avi and Q=0.25-cephalexin.avi, on which all of the analysis has been done.

QuiescentRunTumble.mp4 represents a portion of the video obtained in quiescence. A spotlight is used to highlight two bacteria that are elongated to approximately twice their normal length. Each of these bacteria exhibit run and tumble motion: the first bacteria with a spotlight on it exhibits one or two tumbles; the second spotlighted bacteria exhibits four tumble events through its trajectory.

QuiescentSpotlight.mp4 represents a portion of the video obtained in quiescence in which one bacteria with  $l = 6.94\mu\text{m}$  swims across the field of view for nearly 20 seconds. Its velocity is  $v = 11.03\mu\text{m/s}$  and it wiggles with a frequency  $f_0 = 2.95\text{Hz}$ .

ExampleMethodology.mp4 shows approximately 10s of the raw video obtained in microfluidic flow at  $Q = 0.25\mu\text{L/min}$ . The raw video is followed by a binarized video, demonstrating the image analysis protocol. In both portions of the video, one of the bacteria is marked with a red 'x' at its centroid position. This bacteria has  $l = 5.31\mu\text{m}$ , swims with  $v = 24.3\mu\text{m/s}$ , and wiggles with fundamental frequency  $f_0 = 12.5\text{Hz}$ . Its average orientation is  $\alpha = 85.2^\circ$  and the trajectory direction is  $\beta = 16.2^\circ$ . Several examples of  $\alpha(t)$  over the course of bacteria trajectories are shown in Figure 5.

Upstream1.mp4 and Upstream2.mp4 put spotlights on examples of bacteria that swim upstream next to the wall in  $Q = 0.10\mu\text{L/min}$ . WallAway.mp4 highlights a third bacteria from the same flow rate that both swims upstream near the wall and then swims persistently away from the wall. The velocity of this swimmer as it moves away from the wall is shown in more detail in Figure S8.

## III. SWIMMING IN QUIESCENCE

In quiescence, elongated bacteria swim with an undulatory motion. This can be described by fitting the bacteria shape to a parabola. The concavity of this parabola,  $a$ , can in turn be fit to a sinusoidal function. Figure S2 provides an example of  $a(t)$ , in blue, fitted to  $\sin(f_0 t)$ , overlaid in red. This bacteria is the one highlighted in the QuiescentSpotlight video (with  $v = 11.03\mu\text{m/s}$ ,  $f_0 = 2.95\text{Hz}$ ).

## IV. DEFINING WIGGLING

Figure S3(a) and (b) show examples of the measured shape change of a single bacteria during the course of its trajectory. In both panels, the left axis in blue, of the

\* s.hashmi@northeastern.edu

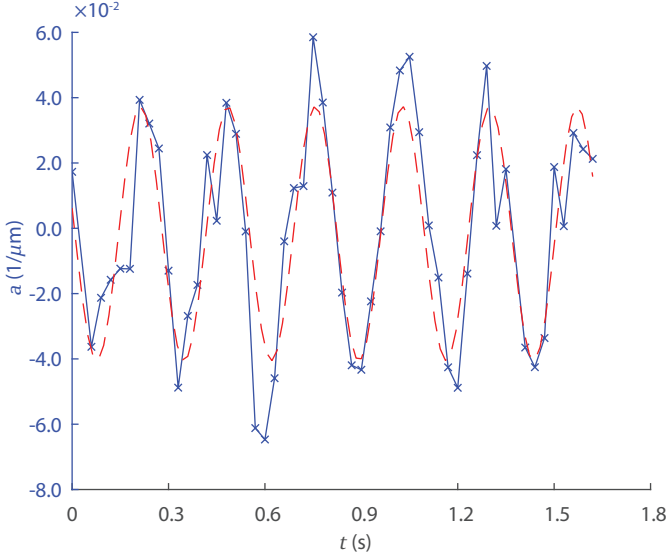

FIG. S2. An elongated swimmer in quiescence exhibits sinusoidal dynamics in the concavity of its shape, traced as a function of time throughout its trajectory.

concavity shape factor  $a$ , and deflection  $\delta$  on the right axis, in green, are plotted as a function of  $t$ . The red dashed lines indicate attempts to fit  $a(t)$  to  $\sin(\omega t)$ .

In Figure S3(a),  $\sin(\omega t)$  fits  $a(t)$  reasonably well, with  $\omega = 8.63$  Hz. This value is within  $< 2\%$  of the fundamental frequency  $f_0 = 8.78$  Hz obtained by the Fourier transform method described in Figure 1. However, out of the total  $\sim 150$  wiggling bacteria measured in both flow rates, only  $\sim 5$  bacteria change shape such that  $a(t)$  is reasonably well described by a sin function in this manner. In Figure S3(b),  $\sin(\omega t)$  does not fit  $a(t)$  well, both as seen by eye and as assessed by R-squared calculations. In this example,  $\omega \sim 1$  Hz, whereas the frequency extracted by the Fourier transform method is  $\sim 10$  times larger. The example in Figure S3(b) is representative of  $> \sim 95\%$  of the wiggling bacteria.

Figures S4 and S5 represent two examples of bacteria which do not meet the criteria for “wiggling” as defined in the manuscript. Panel (a) shows the trajectory of each bacteria. Also, each bacteria exhibits some degree of shape change through its trajectory, as seen in panel (b). However, the Fourier transform analysis reveals that there is no strongly defined  $f_0$ : no frequency has a magnitude  $|P(f)|$  that is more than two standard deviations above the average  $|P(f)|$ . As such, neither of these two example bacteria meet the definition of “wiggling” and are thus classified as “non-wigglers.”

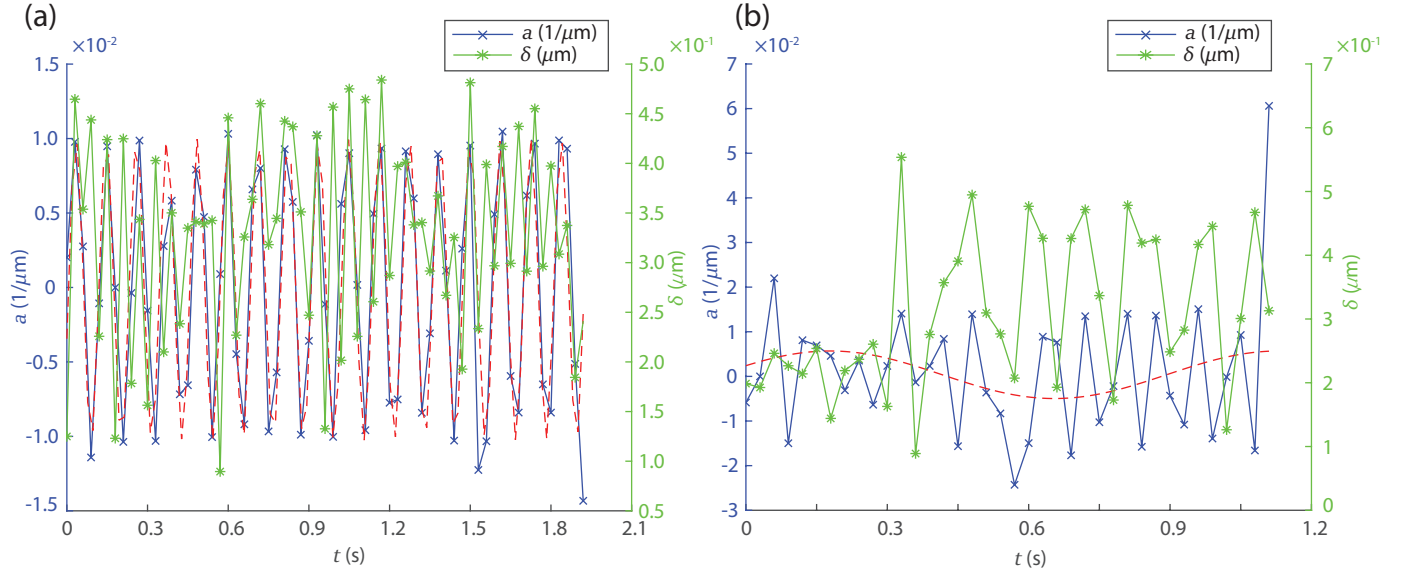

FIG. S3. Two examples of the shape evolution of wiggling bacteria through the course of their trajectories.  $a$ , plotted on the left axis in blue, represents the amplitude of the parabola used to fit the bacteria shape.  $\delta$ , plotted on the right axis in green, represents the deflection. The dashed red line indicates the fit of  $a(t)$  to a sin function  $\sin(\omega t)$ .

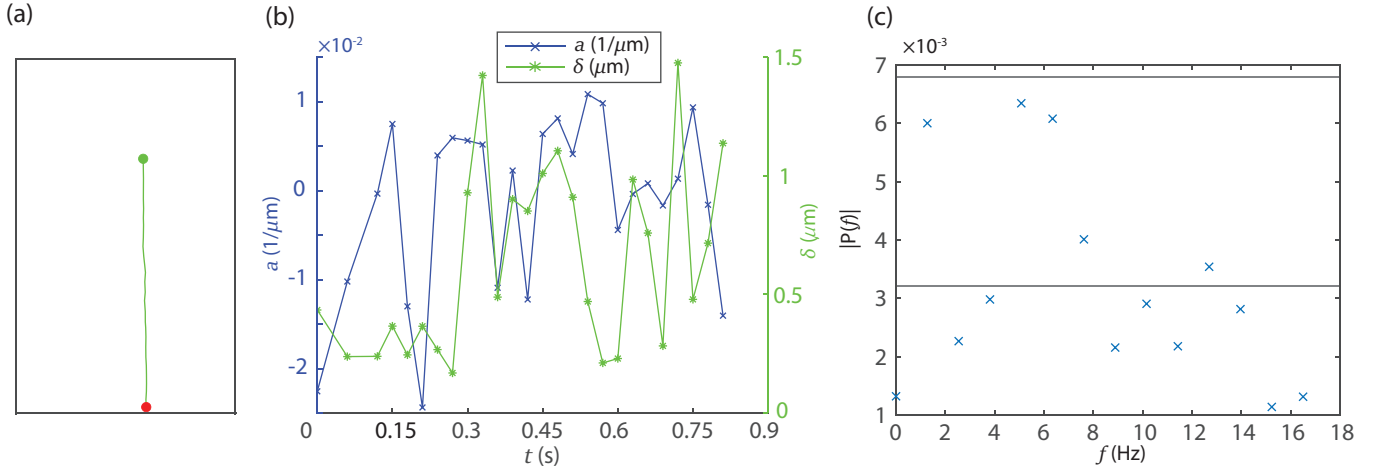

FIG. S4. An example of a bacteria that does not wiggle in flow. (a) shows the trajectory, while (b) and (c) provide the metrics used to define wiggling. In (c), there is no strongly preferred frequency that lies beyond two standard deviations of the average value of  $|P(f)|$ .

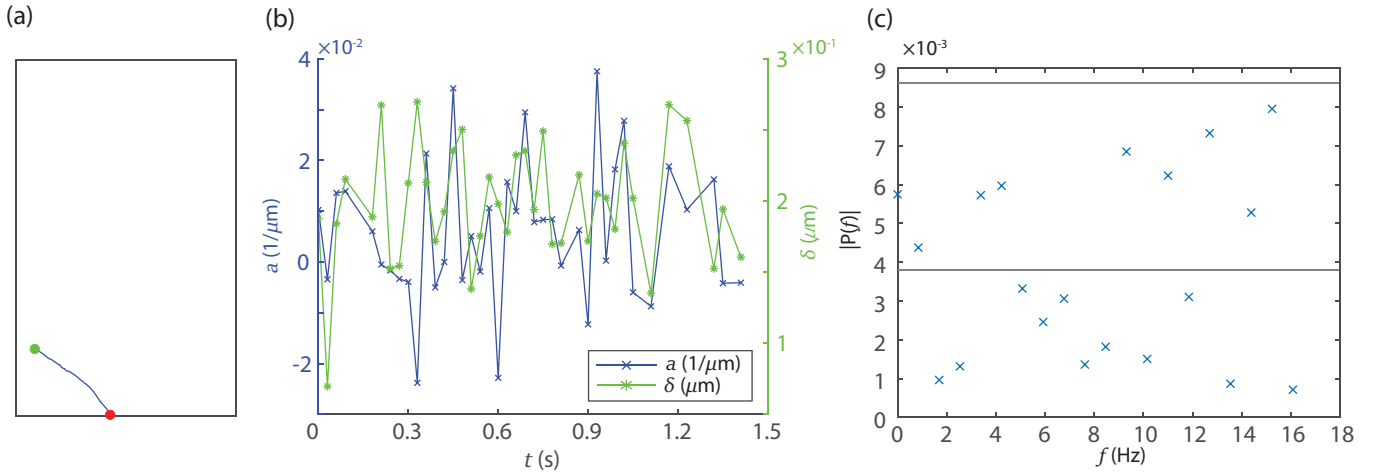

FIG. S5. An example of a bacteria that does not wiggle in flow. (a) shows the trajectory, while (b) and (c) provide the metrics used to define wiggling. Despite curvature in the trajectory shown in (a), (c) indicates there is no strongly preferred frequency that lies beyond two standard deviations of the average value of  $|P(f)|$ .

## V. NON WIGGLERS FOLLOW STREAM LINES

Figure S6 shows the trajectories of the non-wiggling bacteria at each flow rate. The two primary observations in these figures is that the trajectories are both fairly straight,  $\lambda \approx 1$ , and aligned with the streamlines,  $\alpha \sim 0^\circ$ . A few trajectories at the lower flow rate are seen to cross streamlines. These each represent bacteria that wiggle slightly, but not sufficiently enough to meet the definition presented in the manuscript. The example shown in Figures S5 is seen in the lower left corner of Figure S6(a). At the higher flow rate, a few bacteria seem to exhibit a shift in their  $x$  position in the middle of their trajectories. These may represent occasions in which one bacteria collides with another.

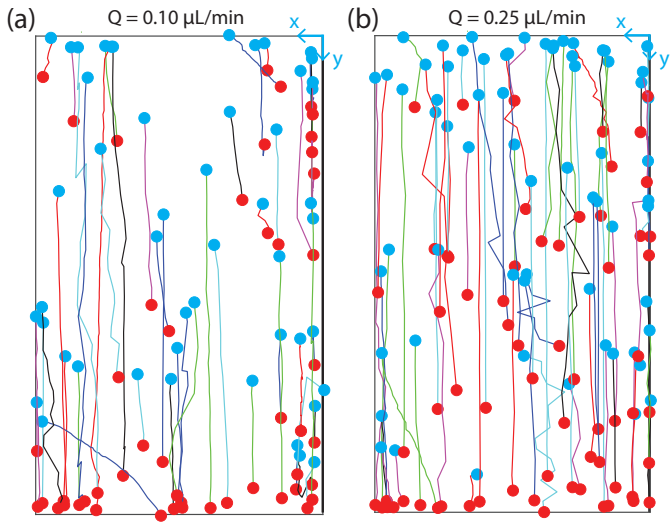

FIG. S6. The above figure captures the trajectories of tracked bacteria that do not exhibit wiggling behavior. The axes are labeled in the upper right corner: the wall is located at  $x = 0\mu\text{m}$  and flow proceeds in the  $y$  direction. The initial position of each trajectory is marked by a blue dot, and the final position by a red dot.

## VI. WIGGLERS TRACE OUT TORTUOUS PATHS

Figure S7 shows the path tortuosities,  $\lambda$  for the wiggling bacteria in the two flow rates. A value of  $\lambda = 1$  indicates that trajectory is exactly linear from the beginning to the end point, with no deviations from the shortest line drawn between those two points. The wiggling bacteria, in flow, trace out more tortuous paths than their non-wiggling counterparts. In the slow flow, these paths are even more tortuous than in the faster flow. That is,  $\lambda$  can be as high as 1.2 in the slow flow, indicating that the trajectory follows a path that is 20% longer than the shortest line between its end points.

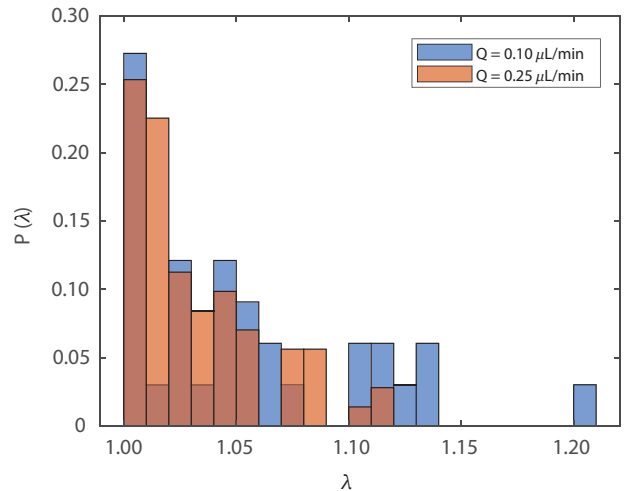

FIG. S7. Histograms of trajectory tortuosity  $\lambda$  for the wigglers in flow, at the two different flow rates.

## VII. ONE BACTERIA SWIMS PERSISTENTLY TOWARD THE CHANNEL CENTER

Figure S8 shows measurements of the instantaneous velocity of the wiggling bacteria that swims persistently away from the wall in the low flow rate,  $Q = 0.10\mu\text{L/min}$ . A video of this swimmer is included in the SI. Its trajectory is seen in Figure 2(a), with its original position in the upper right of the image and its final position in the upper middle of the image. The tracked portion of the trajectory of the bacteria begins near the wall, at  $x \sim 6\mu\text{m}$ , and the bacteria swims toward the center of the channel. Once it reaches  $x \sim 36\mu\text{m}$ , the bacteria leaves the field of view. The example discussed here is the most dramatic example of cross-stream swimming away from the wall. Figure S8(a) shows that the instantaneous velocity  $v$  of this swimmer is roughly constant as a function from its distance from the wall  $x$ . Figures S8(b) and (c) decompose  $v$  into its  $x$  and  $y$  components, respectively.

Notably, the behavior of  $v_x(x)$  seen in Figure S8(b) contrasts passive objects undergoing wall migration. In hydrodynamic wall migration in shear flows, particles which are deformable or non-spherical cross migrate away from walls in an effect sometimes referred to as lift. For passive objects, the cross stream velocity  $v_x$  decreases as the object moves away from the wall, and also scales with the shear rate:  $v_x \sim \dot{\gamma}/x^2$  [1, 2, 3]. In pressure driven flow, the local shear rate  $\dot{\gamma}$  decreases with distance from the wall. In purely parabolic flow,  $\dot{\gamma} \sim 1/x$ , suggesting an even more drastic decrease in  $v_x$  with  $x$ :  $v_x \sim 1/x^3$ . However, as seen in Figure S8(b),  $v_x$  is roughly constant with  $x$ . Figure S8(c) shows  $v_y(x)$  is also relatively constant as the bacteria swims away from the wall. Flow is in the  $y$ -direction, with velocity increasing with  $x$ , toward the center of the channel. Remarkably, the constancy of  $v_y$  suggests that this bacteria is swimming upstream against the fluid, even as the fluid speed increases.

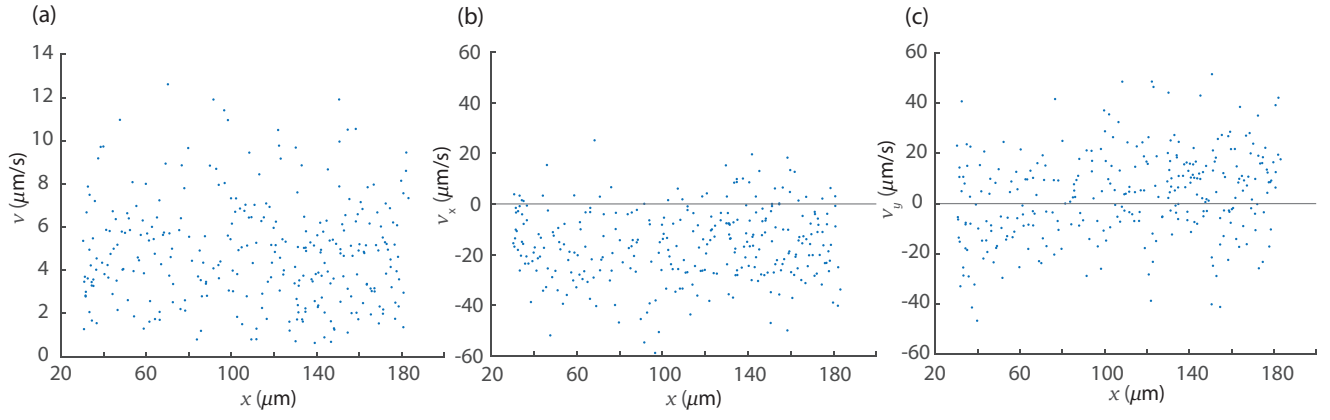

FIG. S8. One wiggling bacteria swims across streamlines at  $Q = 0.10\mu\text{L}/\text{min}$ . Panels (a), (b), and (c) show scatter plots of the instantaneous velocity  $v$  and its  $x$  and  $y$  components, respectively.

### REFERENCES

- [1] PC-H Chan and LG0402 Leal. “The motion of a deformable drop in a second-order fluid”. In: *Journal of fluid mechanics* 92.1 (1979), pp. 131–170.
- [2] Amit Kumar, Rafael G Henríquez Rivera, and Michael D Graham. “Flow-induced segregation in confined multi-component suspensions: effects of particle size and rigidity”. In: *Journal of Fluid Mechanics* 738 (2014), pp. 423–462.
- [3] Sabrina Marnoto and Sara M Hashmi. “Application of droplet migration scaling behavior to microchannel flow measurements”. In: *Soft Matter* 19.3 (2023), pp. 565–573.
